# Supplementary material for: Near-Zero-Shot Suggestion Mining with a Little Help from WordNet
Source: arXiv:2111.12956 source file (2021-11-25)
Supplement: Supplementary file 1 [file 99_appendix.tex]

% \input{tables/messages}

% \begin{table*}[ht]
%     \centering
%     \footnotesize
%         \begin{tabular}{|c|p{.65\linewidth}|cc|}
%         \hline
%          Size &        Labels subset &     F1 & Accuracy \\  \hline
%          \multirow{3}{*}{4} & direction or instruction,proposal,reminder,request or petition or postulation & 0.6590 &   0.6976 \\
%          &  direction or instruction,promotion or publicity or promotional\_material or packaging,proposal,request or petition or postulation & 0.6589 &   0.7027 \\
%          &    direction or instruction,guidance or counsel or counseling or counselling or direction,promotion or publicity or promotional\_material or packaging,proposal & 0.6562 &   0.7027 \\ \hline
%             \multirow{3}{*}{5} &                                                                                                    direction or instruction,guidance or counsel or counseling or counselling or direction,proposal,reminder,request or petition or postulation & 0.6654 &   0.7010 \\
%              &                                                 direction or instruction,guidance or counsel or counseling or counselling or direction,promotion or publicity or promotional\_material or packaging,proposal,request or petition or postulation & 0.6654 &   0.7061 \\
%              &                                                                                                      direction or instruction,promotion or publicity or promotional\_material or packaging,proposal,reminder,request or petition or postulation & 0.6642 &   0.6993 \\ \hline
%             \multirow{3}{*}{6} &                                        direction or instruction,guidance or counsel or counseling or counselling or direction,promotion or publicity or promotional\_material or packaging,proposal,reminder,request or petition or postulation & 0.6704 &   0.7027 \\
%              &                             direction or instruction,guidance or counsel or counseling or counselling or direction,promotion or publicity or promotional\_material or packaging,proposal,request or petition or postulation,submission or entry & 0.6679 &   0.7078 \\
%              &                                                                                direction or instruction,guidance or counsel or counseling or counselling or direction,proposal,reminder,request or petition or postulation,submission or entry & 0.6679 &   0.7027 \\ \hline
%             \multirow{3}{*}{7} &                    direction or instruction,guidance or counsel or counseling or counselling or direction,promotion or publicity or promotional\_material or packaging,proposal,reminder,request or petition or postulation,submission or entry & 0.6729 &   0.7044 \\
%              &                      direction or instruction,guidance or counsel or counseling or counselling or direction,offer or offering,promotion or publicity or promotional\_material or packaging,proposal,reminder,request or petition or postulation & 0.6704 &   0.6993 \\
%              &           direction or instruction,guidance or counsel or counseling or counselling or direction,offer or offering,promotion or publicity or promotional\_material or packaging,proposal,request or petition or postulation,submission or entry & 0.6679 &   0.7044 \\ \hline
%             8 &  direction or instruction,guidance or counsel or counseling or counselling or direction,offer or offering,promotion or publicity or promotional\_material or packaging,proposal,reminder,request or petition or postulation,submission or entry & 0.6728 &   0.7010 \\
%         \hline
%         \end{tabular}

%     \caption{Development set. Top-3 label (all lemmas concatenated with ``or'') subsets results for each subset size from 5 to 8 selected by F1 measure.}
%     \label{tab:my_label}
% \end{table*}

% % \begin{table*}[h]
% %     \centering
% %     \begin{tabular}{|c|r|cc|} \hline
% %         Size &   Labels subset &     F$1$ & Accuracy \\ \hline
% %         \multirow{3}{*}{4} &                                      guidance,promotion,proposal,request & \textbf{0.4955} &   0.8655 \\
% %          &                                      direction,guidance,proposal,request & 0.4825 &   0.8583 \\
% %          &                                     direction,promotion,proposal,request & 0.4818 &   0.8631 \\ \hline
% %         \multirow{3}{*}{5} &                                guidance,offer,promotion,proposal,request & 0.4745 &   0.8271 \\
% %          &                            direction,guidance,promotion,proposal,request & 0.4741 &   0.8535 \\
% %          &                                direction,guidance,offer,proposal,request & 0.4643 &   0.8199 \\ \hline
% %         \multirow{3}{*}{6} &                      direction,guidance,offer,promotion,proposal,request & 0.4577 &   0.8151 \\
% %          &                     guidance,offer,promotion,proposal,request,submission & 0.4475 &   0.8043 \\
% %          &                 direction,guidance,promotion,proposal,request,submission & 0.4427 &   0.8307 \\ \hline
% %         \multirow{3}{*}{7} &           direction,guidance,offer,promotion,proposal,request,submission & 0.4328 &   0.7923 \\
% %          &             direction,guidance,offer,promotion,proposal,reminder,request & 0.4237 &   0.7779 \\
% %          &            guidance,offer,promotion,proposal,reminder,request,submission & 0.4157 &   0.7671 \\ \hline
% %         {8} &  (all $8$ labels) & 0.4035 &   0.7551 \\ \hline
% %     \end{tabular}
% %     \label{tab:test_a_top_3}
% %     \caption{Test set, task A. Top-3 label subsets results for each subset size from $4$ to $8$ selected by F1 measure.}
% % \end{table*}

% \begin{table*}[h]
%     \centering
%     \begin{tabular}{|c|r|cc|} \hline
% % \toprule
%  size &                                                                   subset &     f1 & accuracy \\  \hline
% % \midrule
%     % \multirow{3}{*}{3} &                                                  offer,proposal,reminder & 0.6725 &   0.7240 \\
%     %  &                                                  guidance,offer,reminder & 0.6578 &   0.7129 \\
%     %  &                                                   offer,reminder,request & 0.6538 &   0.7104 \\  \hline
%     \multirow{3}{*}{4} &                                         guidance,offer,proposal,reminder & 0.6934 &   0.7351 \\
%      &                                          offer,proposal,reminder,request & 0.6897 &   0.7327 \\
%      &                                        direction,offer,proposal,reminder & 0.6802 &   0.7277 \\  \hline
%     \multirow{3}{*}{5} &                                 guidance,offer,proposal,reminder,request & 0.7097 &   0.7438 \\
%      &                               direction,guidance,offer,proposal,reminder & 0.7007 &   0.7389 \\
%      &                                direction,offer,proposal,reminder,request & 0.6970 &   0.7364 \\  \hline
%     \multirow{3}{*}{6} &                       direction,guidance,offer,proposal,reminder,request & 0.7167 &   0.7475 \\
%      &                      guidance,offer,proposal,reminder,request,submission & 0.7123 &   0.7450 \\
%      &                       guidance,offer,promotion,proposal,reminder,request & 0.7067 &   0.7401 \\  \hline
%     \multirow{3}{*}{7} &            direction,guidance,offer,proposal,reminder,request,submission & \textbf{0.7192} &   0.7488 \\
%      &             direction,guidance,offer,promotion,proposal,reminder,request & 0.7137 &   0.7438 \\
%      &            guidance,offer,promotion,proposal,reminder,request,submission & 0.7093 &   0.7413 \\  \hline
%     8 &  (all 8 labels) & 0.7163 &   0.7450 \\  \hline
% % \bottomrule
% \end{tabular}
%     \label{tab:dev_b_top_3}
%     \caption{Dev set, Subtask B. Top-3 label subsets results for each subset size from $4$ to $8$ selected by F1 measure.}
% \end{table*}

% \begin{table*}[h]
%     \centering
%     \begin{tabular}{|c|r|cc|} \hline
% % \toprule
%  size &                                                                   subset &     f1 & accuracy \\  \hline
% % \midrule
%     % \multirow{3}{*}{3} &                                                  offer,proposal,reminder & 0.5759 &   0.6748 \\
%     %  &                                                   offer,reminder,request & 0.5669 &   0.6699 \\
%     %  &                                                  guidance,offer,reminder & 0.5538 &   0.6578 \\ \hline 
%     \multirow{3}{*}{4} &                                          offer,proposal,reminder,request & 0.5963 &   0.6845 \\
%      &                                         guidance,offer,proposal,reminder & 0.5833 &   0.6723 \\
%      &                                        offer,promotion,proposal,reminder & 0.5804 &   0.6772 \\ \hline
%     \multirow{3}{*}{5} &                                 guidance,offer,proposal,reminder,request & 0.6030 &   0.6820 \\
%      &                                offer,promotion,proposal,reminder,request & 0.6006 &   0.6869 \\
%      &                               offer,proposal,reminder,request,submission & 0.5997 &   0.6857 \\ \hline
%     \multirow{3}{*}{6} &                       guidance,offer,promotion,proposal,reminder,request & 0.6073 &   0.6845 \\
%      &                      guidance,offer,proposal,reminder,request,submission & 0.6063 &   0.6833 \\
%      &                       direction,guidance,offer,proposal,reminder,request & 0.6054 &   0.6820 \\ \hline
%     \multirow{3}{*}{7} &            guidance,offer,promotion,proposal,reminder,request,submission & 0.6105 &   0.6857 \\
%      &             direction,guidance,offer,promotion,proposal,reminder,request & 0.6096 &   0.6845 \\
%      &            direction,guidance,offer,proposal,reminder,request,submission & 0.6087 &   0.6833 \\ \hline
%     8 &  (all $8$ labels) & \textbf{0.6129} &   0.6857 \\
%  \hline
% \end{tabular}
%     \label{tab:test_b_top_3}
%     \caption{Test set, Subtask B. Top-3 label subsets results for each subset size from $4$ to $8$ selected by F1 measure.}
% \end{table*}
